# Supplementary material for: Navigating the Trade-Off between Multi-Task Learning and Learning to Multitask in Deep Neural Networks
Source: arXiv:2007.10527 source file (2021-01-05)
Supplement: Supplementary file 1 [file supplementary.tex]

\section{Supplementary Material}

\subsection{Experimental Details}
Our data consists of $29,250$ data-points generated in AirSim. Each data-point consists of examples for each input (GPS and image) and labels for all four tasks. The GPS-input is a two-dimensional input whereas the image-input is $84 \times 84$.

The specific network architecture we use involves processing the GPS-input using a single-layer neural network with $50$ hidden units and image-input using a $4$-layer convolutional network with $32$ feature maps in each layer. The final hidden-layer representations for each type of network are then mapped to the different outputs using a fully-connected layer. All networks are trained using SGD with learning rate of $0.1$ that is decayed across the trials. At each trial, the network receives $160$ items for which it is trained on all $4$ tasks either via single-tasking or multitasking. For single-tasking, the network is trained on each task one after another, where the data for each task is treated as one mini-batch. For multitasking, the network is trained on performing Tasks $1$ and $4$ concurrently and then on performing Tasks $2$ and $3$ concurrently, where again data for each multitasking execution is treated as one mini-batch. We measure the learning speed for each task by measuring the accuracy on the data for a task before the network is updated to be trained on that data. For the results shown in Figures $4$ and $5$ in the main text, the networks are trained for $20,000$ trials. The error bars represent $95 \%$ confidence intervals computed using $10$ different network initializations, where each initialization involves using a different random seed when sampling weights according to the Xavier initialization scheme for both convolutional and fully-connected layers. Lastly, all models were trained on a Nvidia Titan X GPU.

The multitasking error for a network is computed by measuring how much worse the average performance for all the data for a task is when the task is executed in multitasking fashion vs when it is executed as a single task. Thus, for example, to get the multitasking error for Task $1$, we would measure the error in average performance when executing the task in multitasking fashion (where we execute Tasks $1$ and $4$ concurrently) vs executing the task just by itself.

The amount of sharing of representations between two tasks is computed by taking the average representations for the two tasks (when executed in single-tasking fashion) across all the data and measuring the correlation between these two average representations. We can compute this layer-wise by only considering the average representation at a certain layer.

\subsection{Meta-Learning Experimental Details}
Information about hyper-parameters used for meta-learning are shown in Table~\ref{table:hyperparam}. The hyper-parameters for number of particles and posterior re-computation were primarily picked to have a feasible running-time whereas the prior parameters were picked to be representative of a reward function that was non-decreasing over time and converging to perfect performance by the end of the total number of trials. The error bars in Figure $6$a and $6$b represent $95 \%$ confidence intervals computed using $15$ different runs of the meta-learner.

\begin{table}[t]
\centering
\begin{tabular}{|c|c|}
\hline
Hyper-parameter Description & Value \\
\hline 
\hline
Number of Particles for SVGD & $5$ \\ \hline
\shortstack{Amount of new trial data \\ to re-compute posterior} & $50$ \\ \hline
Prior distribution for $w_1$ & $\mathcal{N}(0.001, 0.2)$ \\ \hline
Prior distribution for $w_2$ & $\mathcal{N}(10, 1)$ \\ \hline
Prior distribution for $b_1$ & $\mathcal{N}(-2, 1)$ \\ \hline
Prior distribution for $b_2$ & $\mathcal{N}(-5, 1)$ \\ \hline
\end{tabular}
\caption{Hyper-parameters for meta-learning.}
\label{table:hyperparam}
\end{table}

\subsection{Visualization of Multitasking Error}
Figure~\ref{fig:multierrorvis} visualizes the outputs of a single-tasking trained and a multitasking trained network asked to perform Task $1$ (GPS-localization) and Task $4$ (Image-classification) concurrently. The examples show mis-classifications by the single-tasking trained network on Task $1$ when multitasking, as the single-tasking trained network seems to err towards the output of Task $3$ (Image-localization). Executing Task $1$ and $4$ requires activation of representations for both tasks in the hidden layers by the task-input layer. This leads to an implicit engagement of Task $3$ which shares a representation with Task $4$, leading to cross-talk with Task $1$ at the location output layer. In these examples, we see that the prediction for the GPS location is biased toward the location of the object which would correspond to the correct label for the implicitly activated Task $3$. The multitasking trained network, on the other hand, does not suffer from this cross-talk and is able to execute Tasks $1$ and $4$ concurrently with no error.

\begin{figure}[t]
    \centering
    \includegraphics[width=0.8\linewidth]{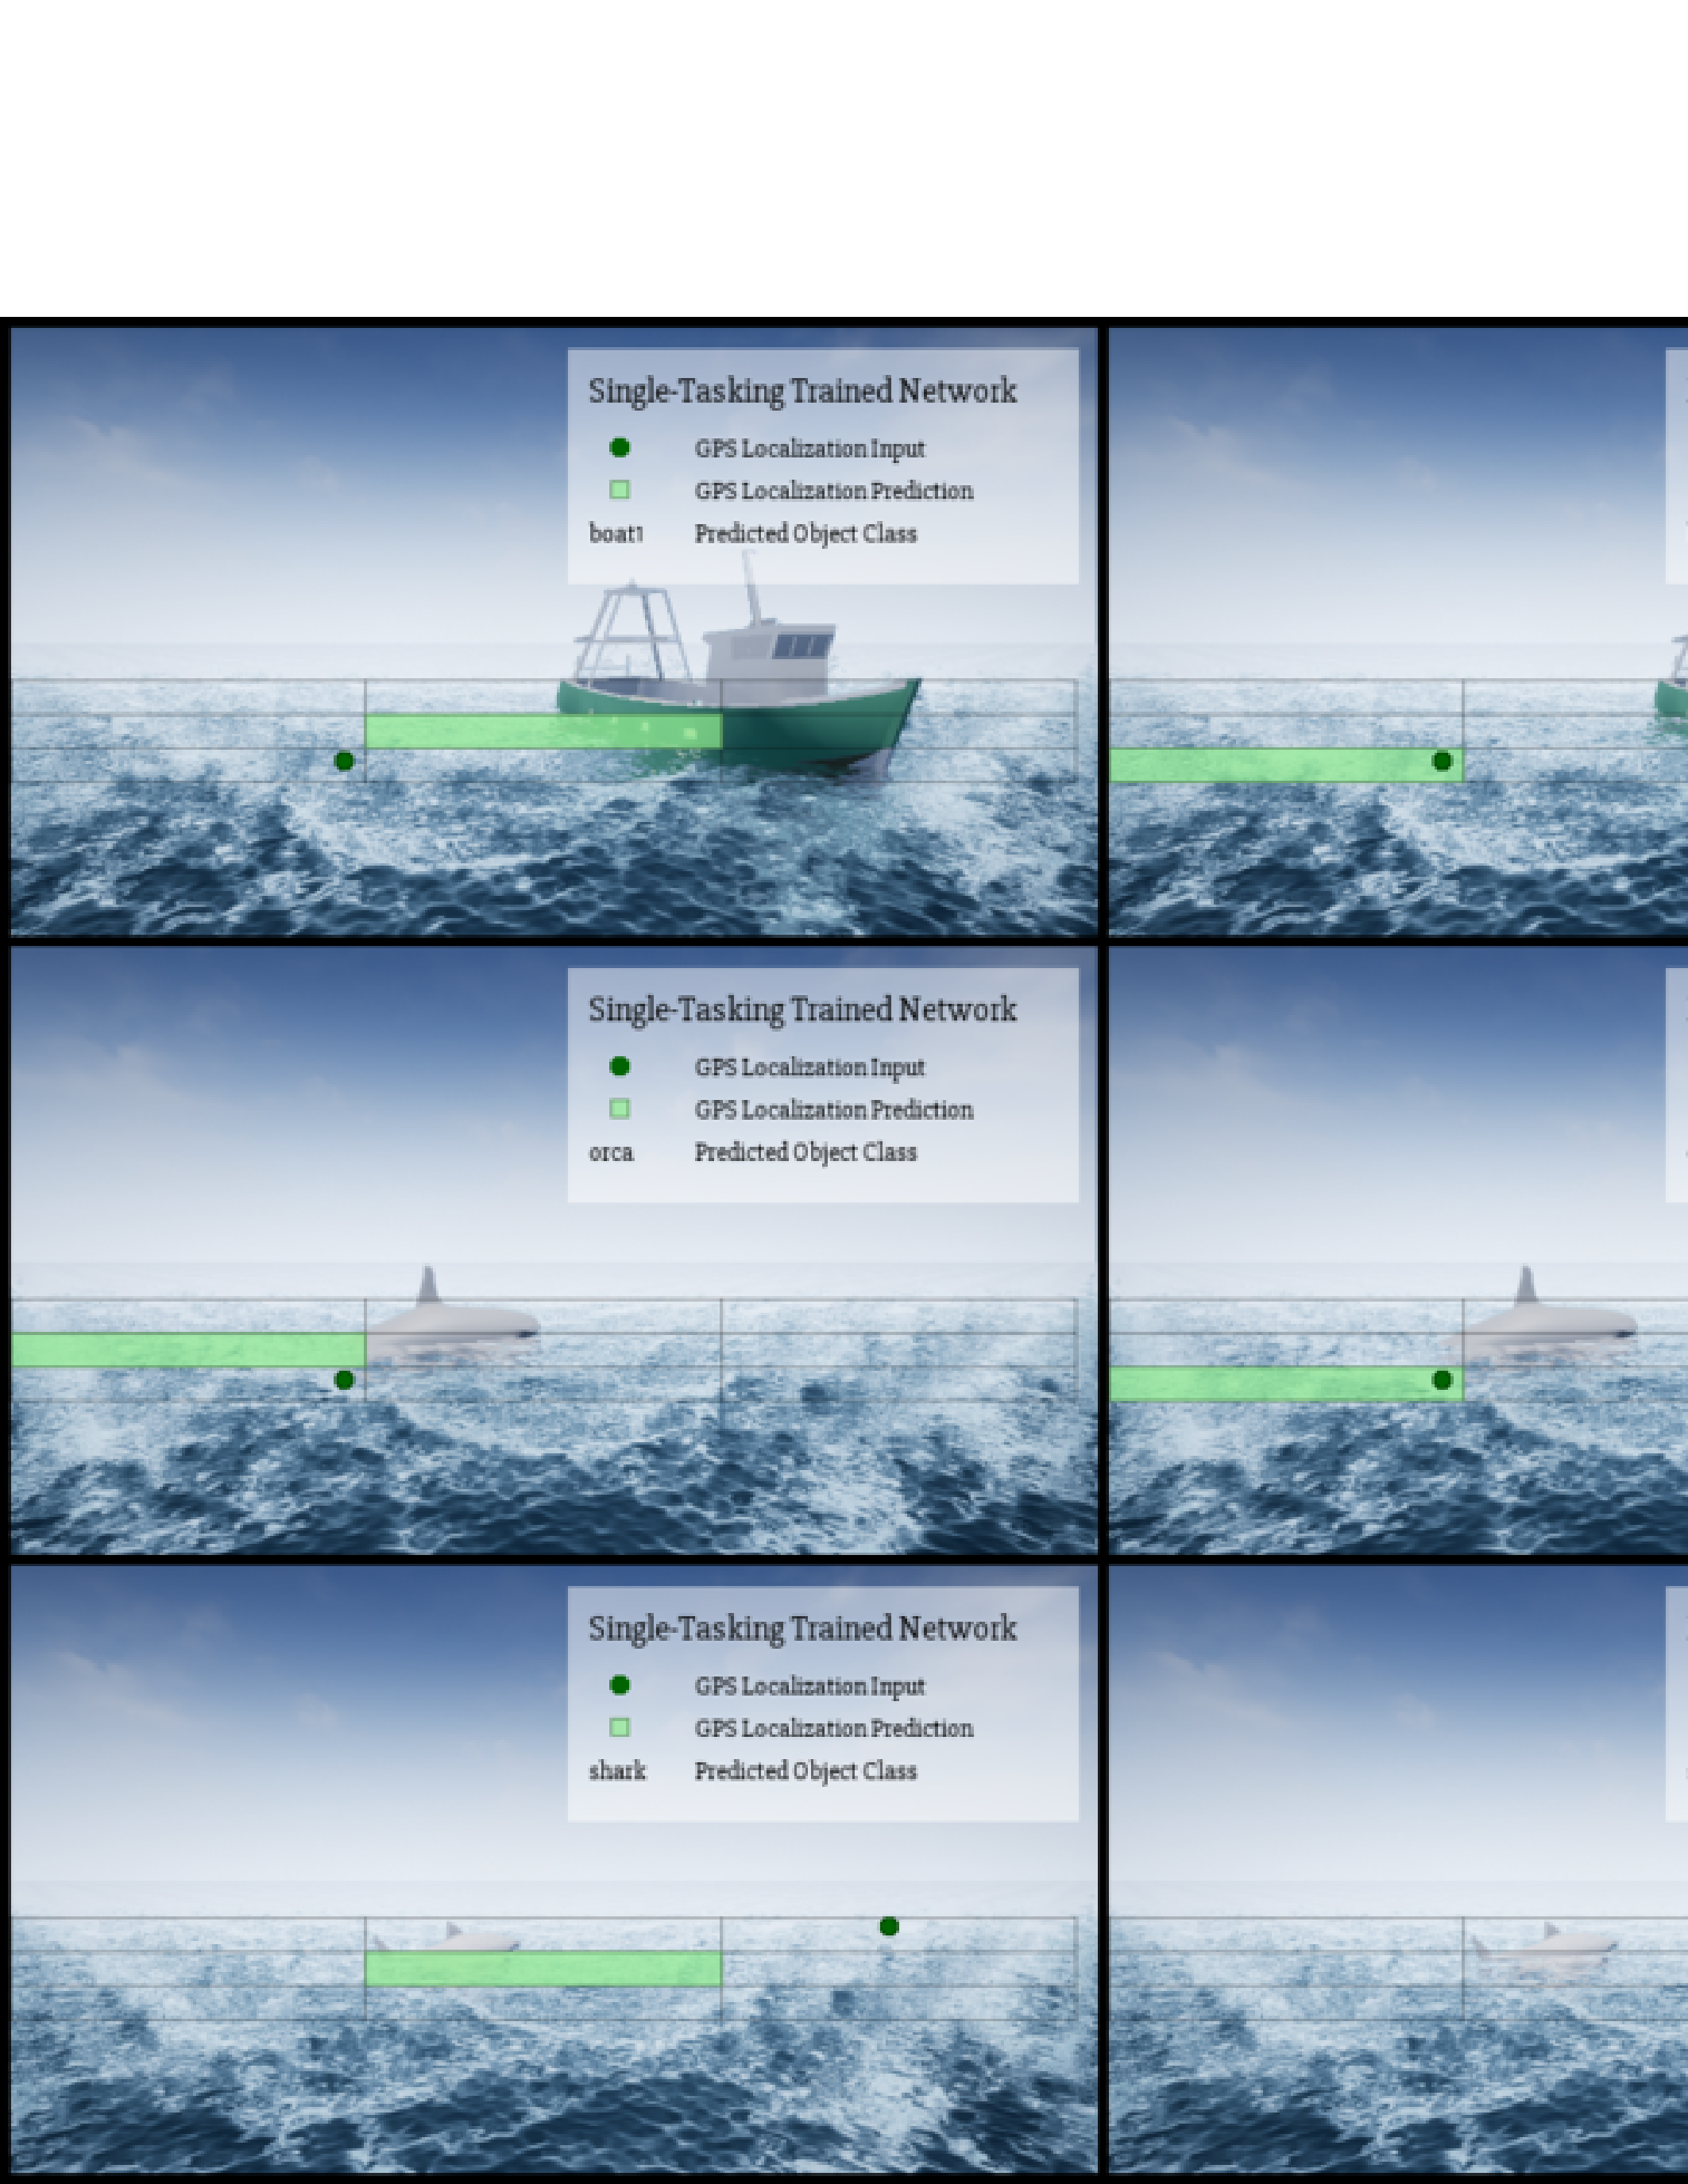}
    \caption{Visualization of predictions from concurrent execution of Tasks 1 and 4 in a single-tasking trained (left) and multitasking trained (right) network. For a correct output for Task 1 (GPS-localization), the predicted output (green box) should contain the GPS-input (green point).}
    \label{fig:multierrorvis}
\end{figure}

\subsection{Effect of Sharing Representations on Learning Speed and Multitasking Ability with Different Initialization}
In Figure~\ref{fig:multitask_diff_init}, we show results comparing single-task vs multitask training when the network isn't as biased towards using shared representations because of initialization using smaller task-associated weights. We see the same conclusions as the previous related experiment in the main text; however, the learning speed benefit of the single-task trained network seems even larger in this case.

\begingroup
\makeatletter
\renewcommand{\p@subfigure}{}% Void parent macro for figures
\begin{figure}
    \centering
    % 0.53
    \begin{subfigure}[b]{.38\textwidth}
      \centering
      \includegraphics[width=1.15\linewidth]{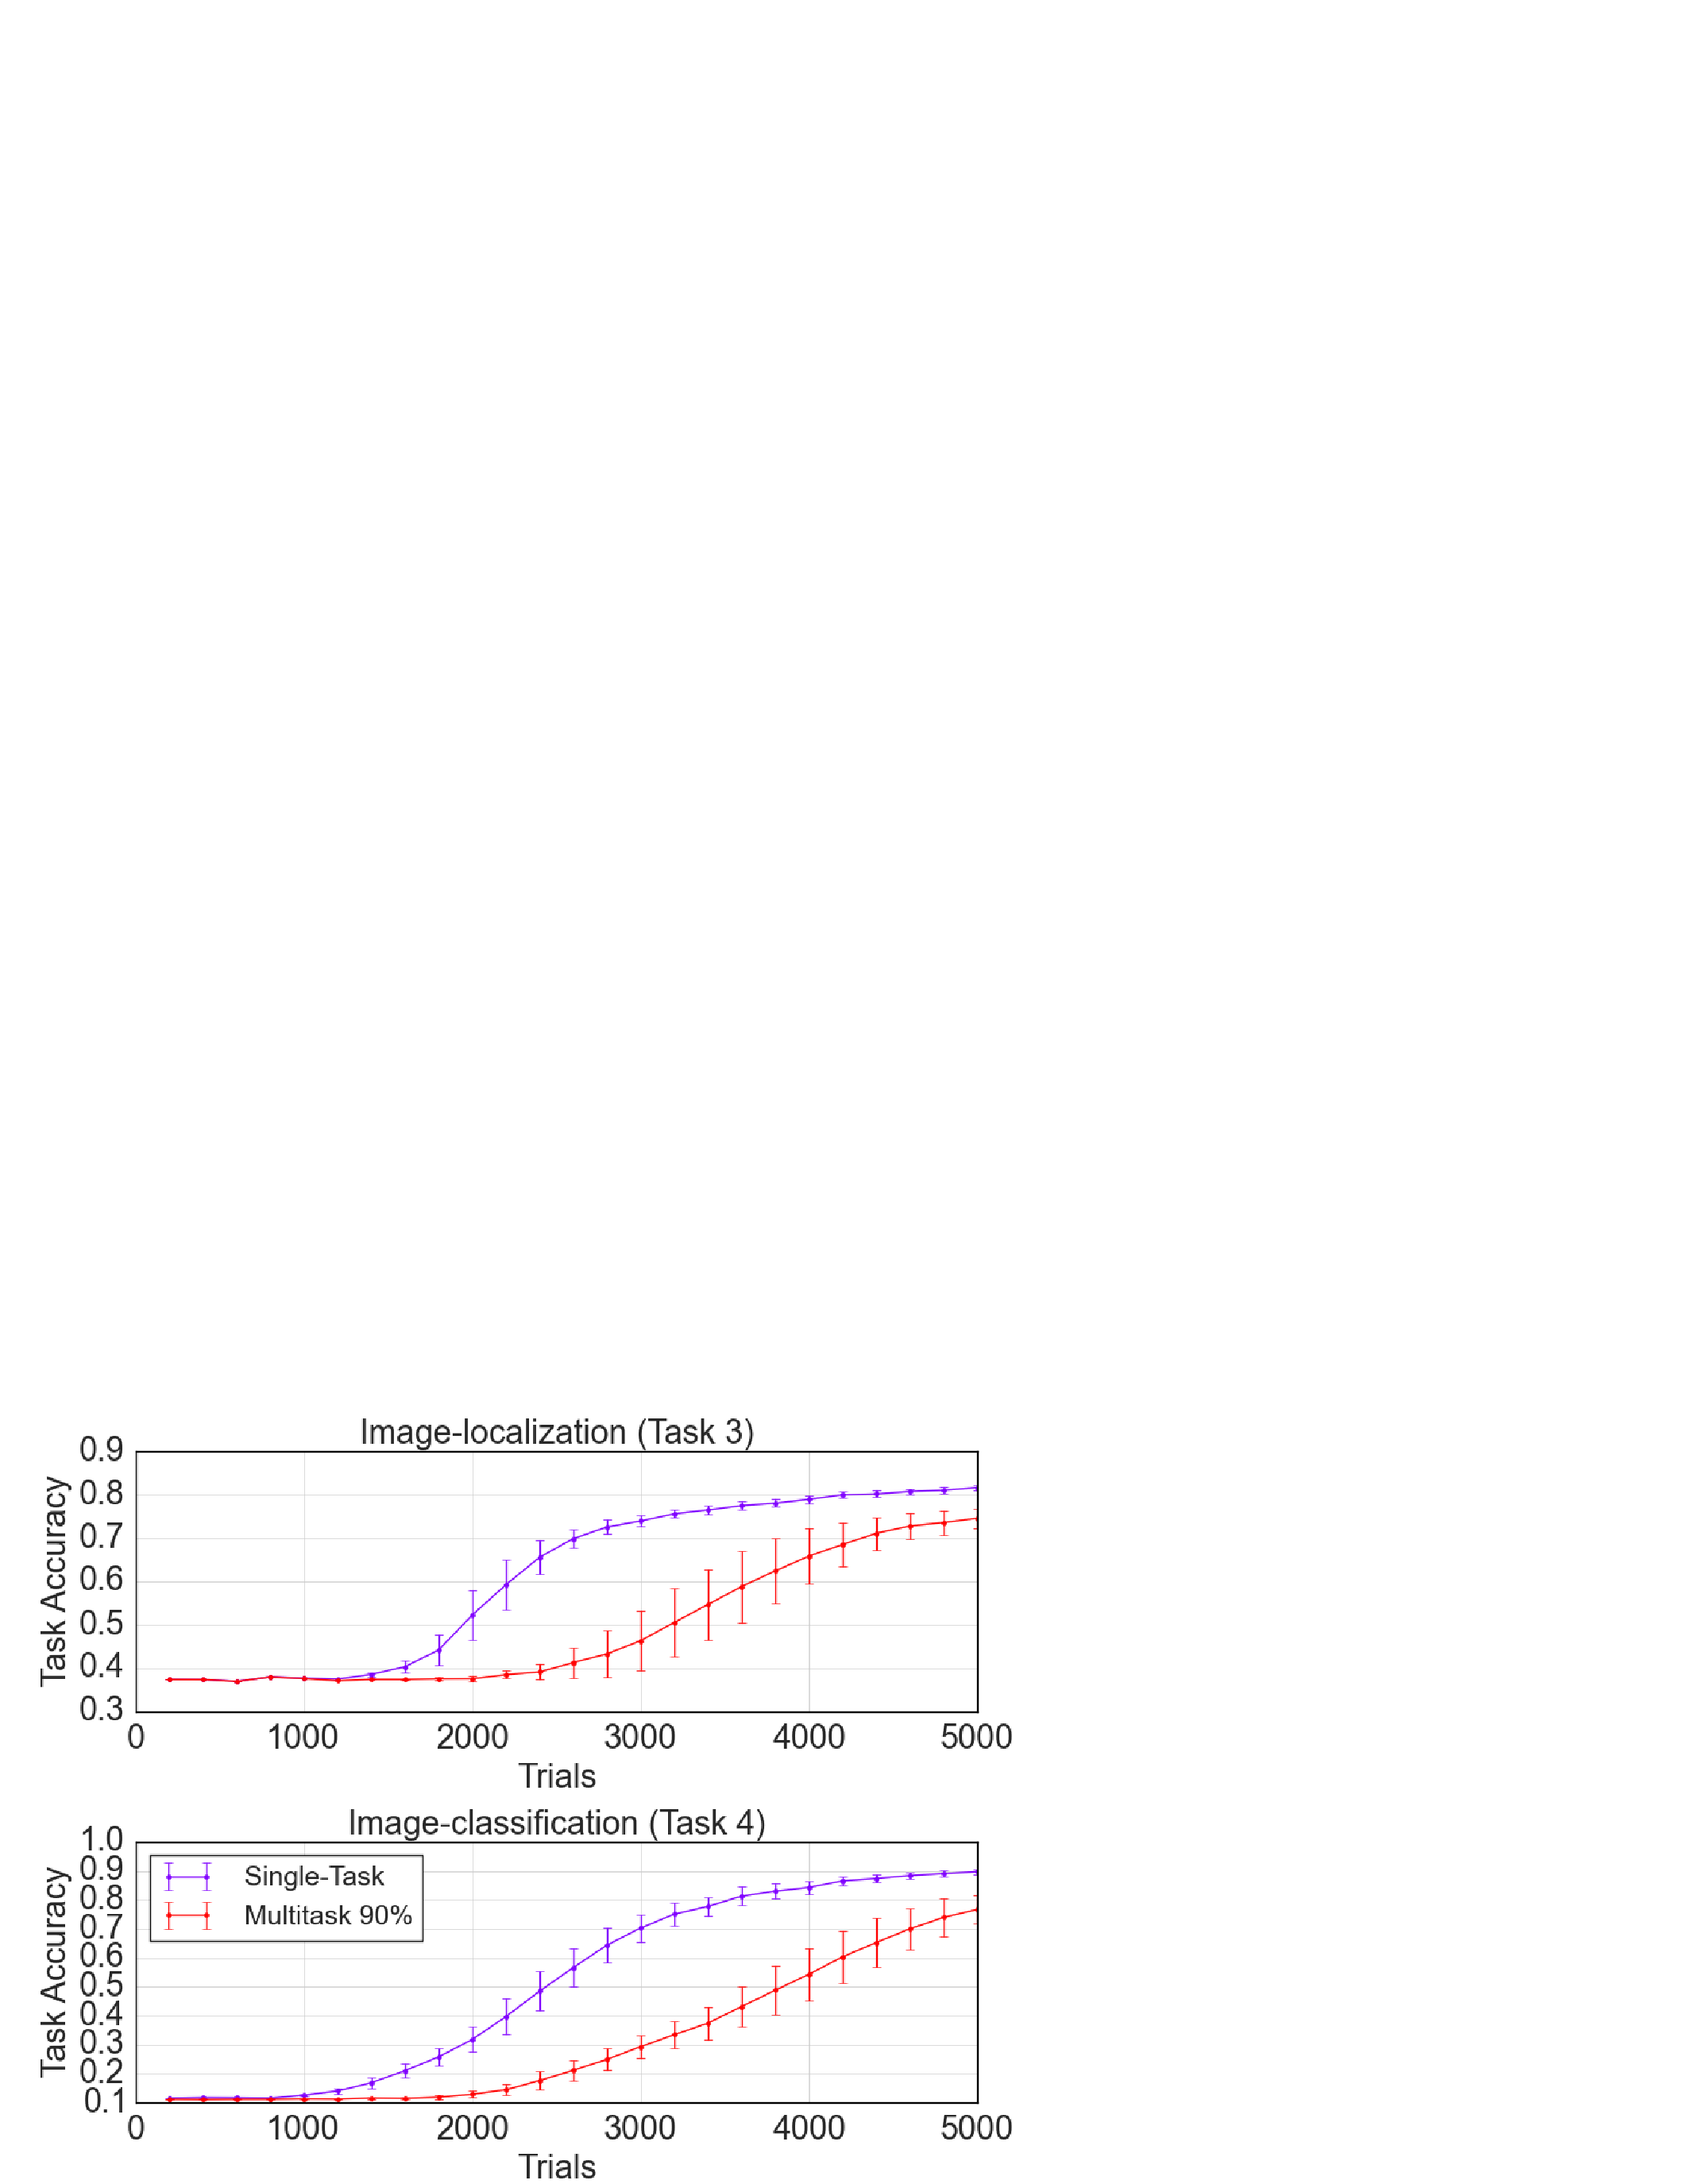}
      \caption{}
      \label{fig:multitask_learning_speed}
    \end{subfigure}
    % 0.46
    \begin{subfigure}[b]{0.34\textwidth}
        \centering
        \begin{minipage}[b]{0.55\textwidth}
            \centering
            \includegraphics[width=\textwidth]{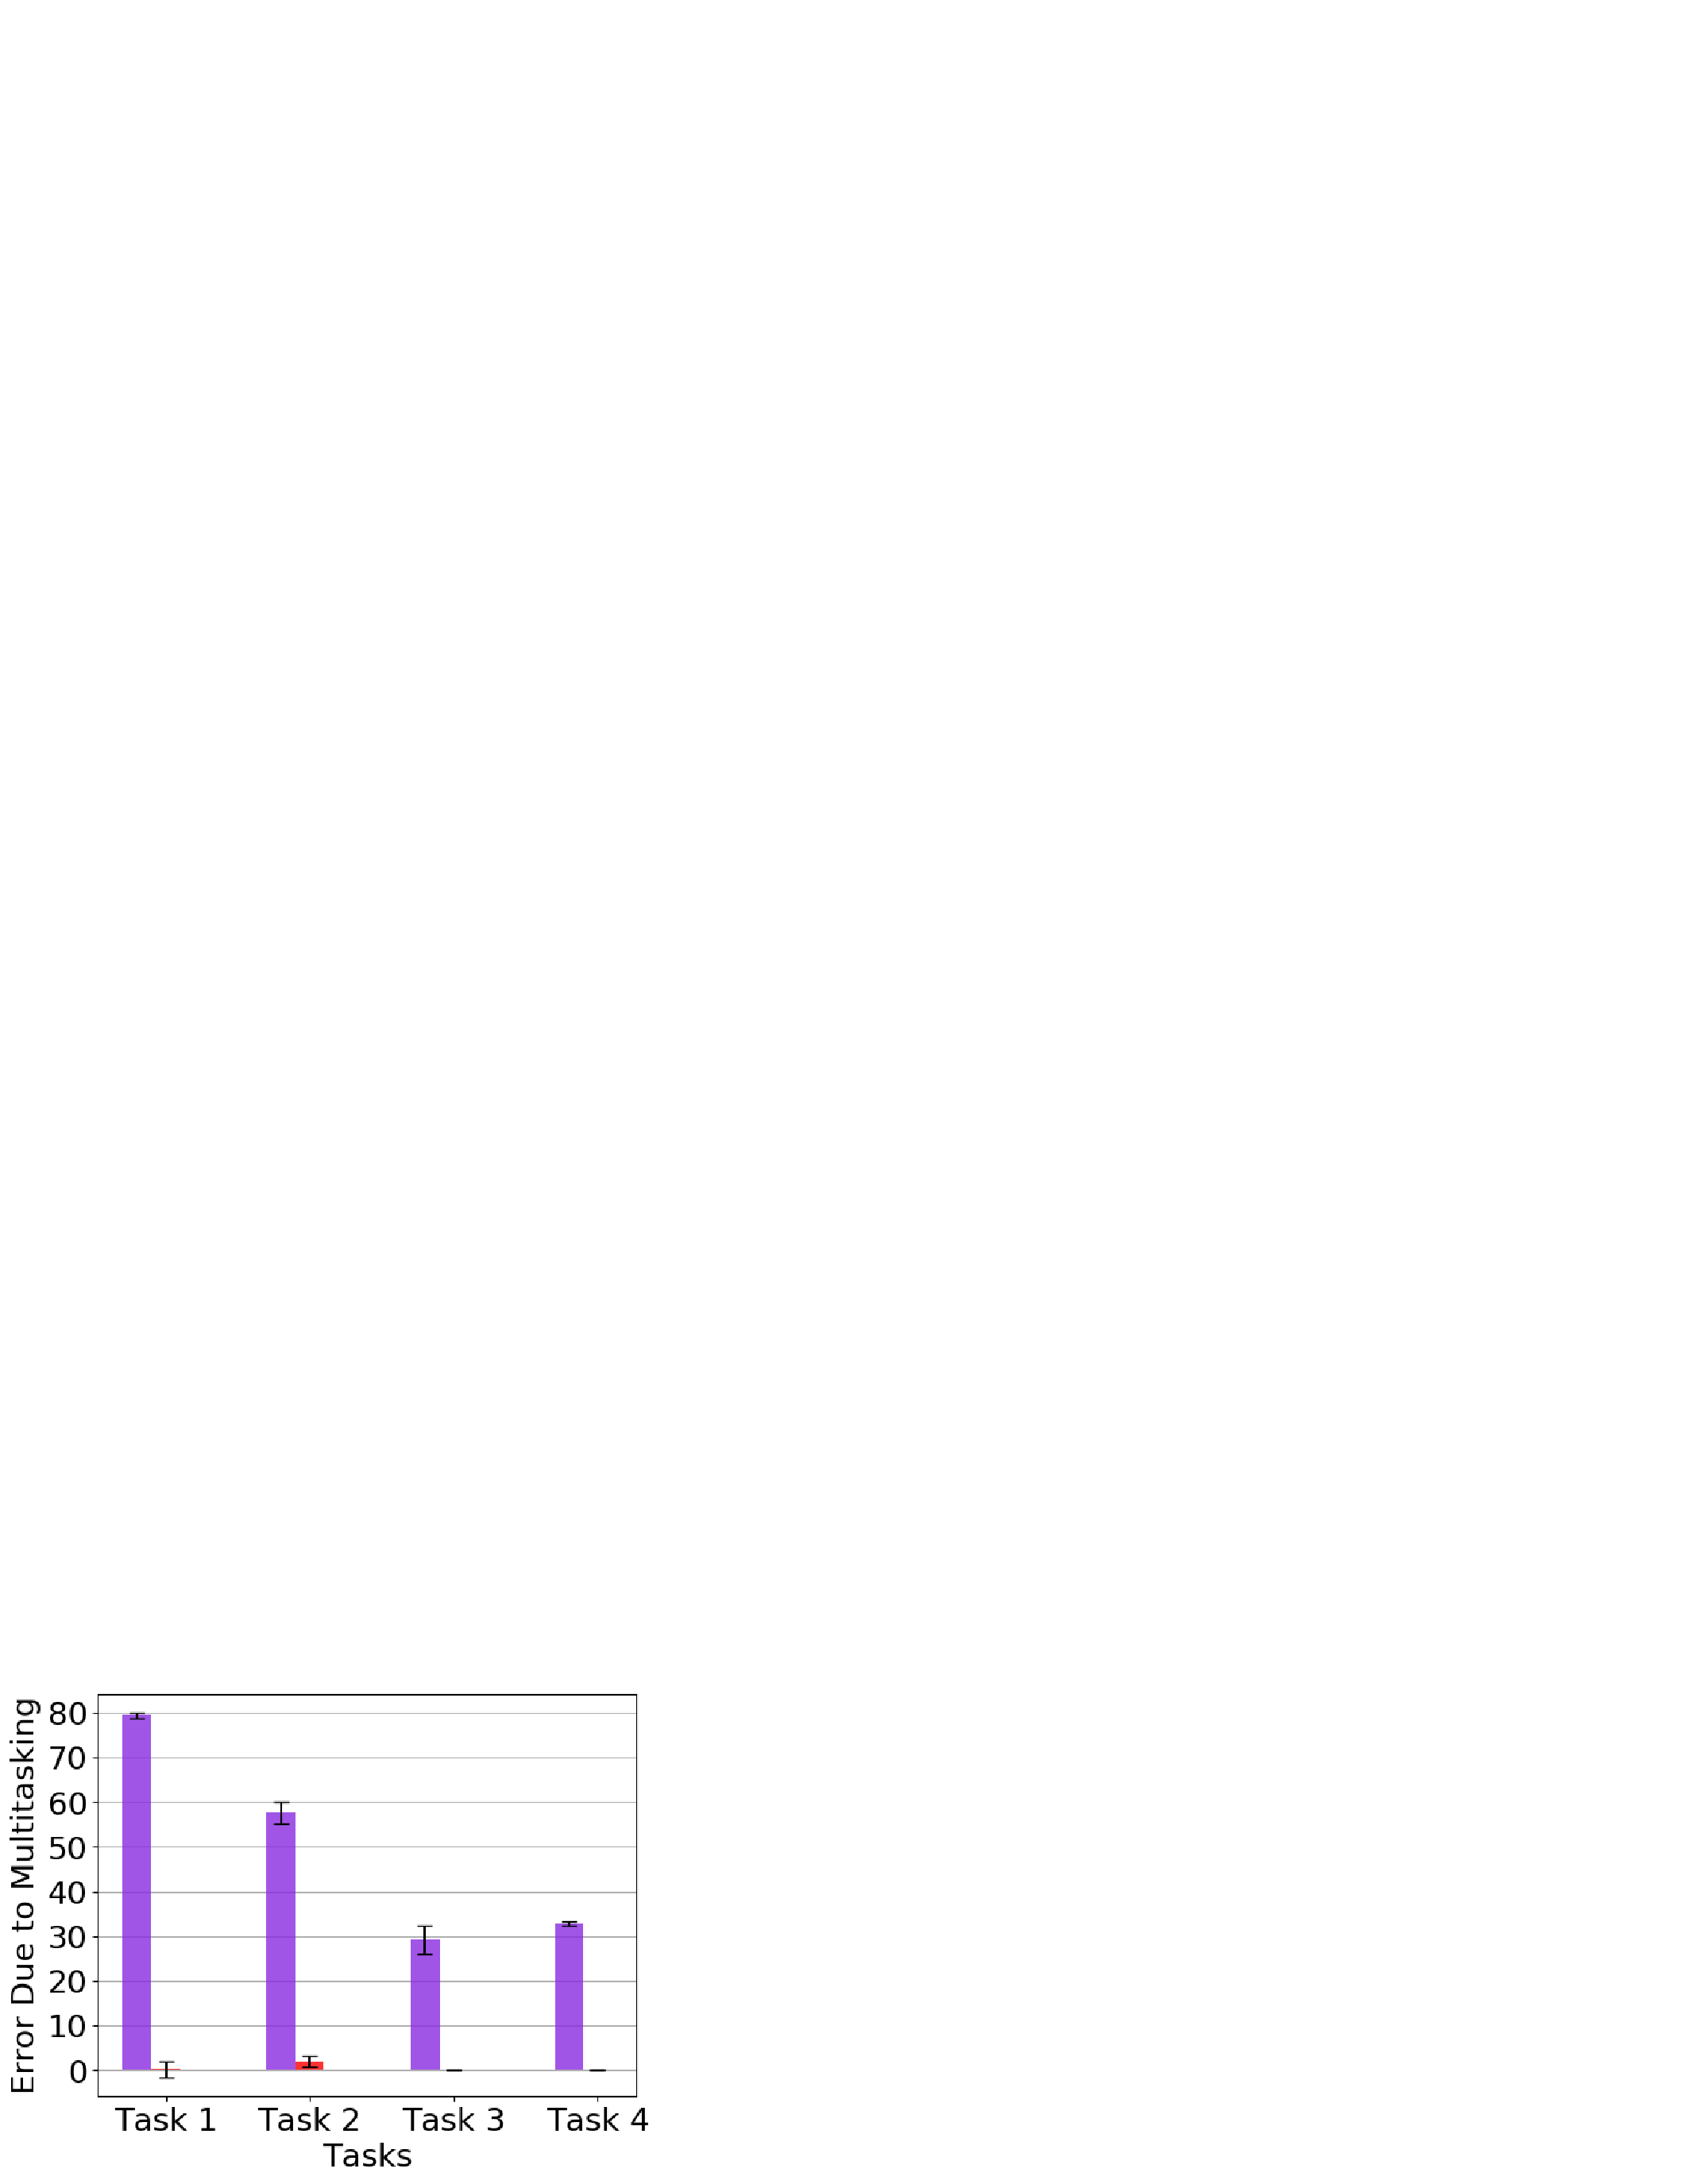}
            \caption{}
            \label{fig:multitask_error}
        \end{minipage}
        \begin{minipage}[b]{0.55\textwidth}
            \centering
            \includegraphics[width=\textwidth]{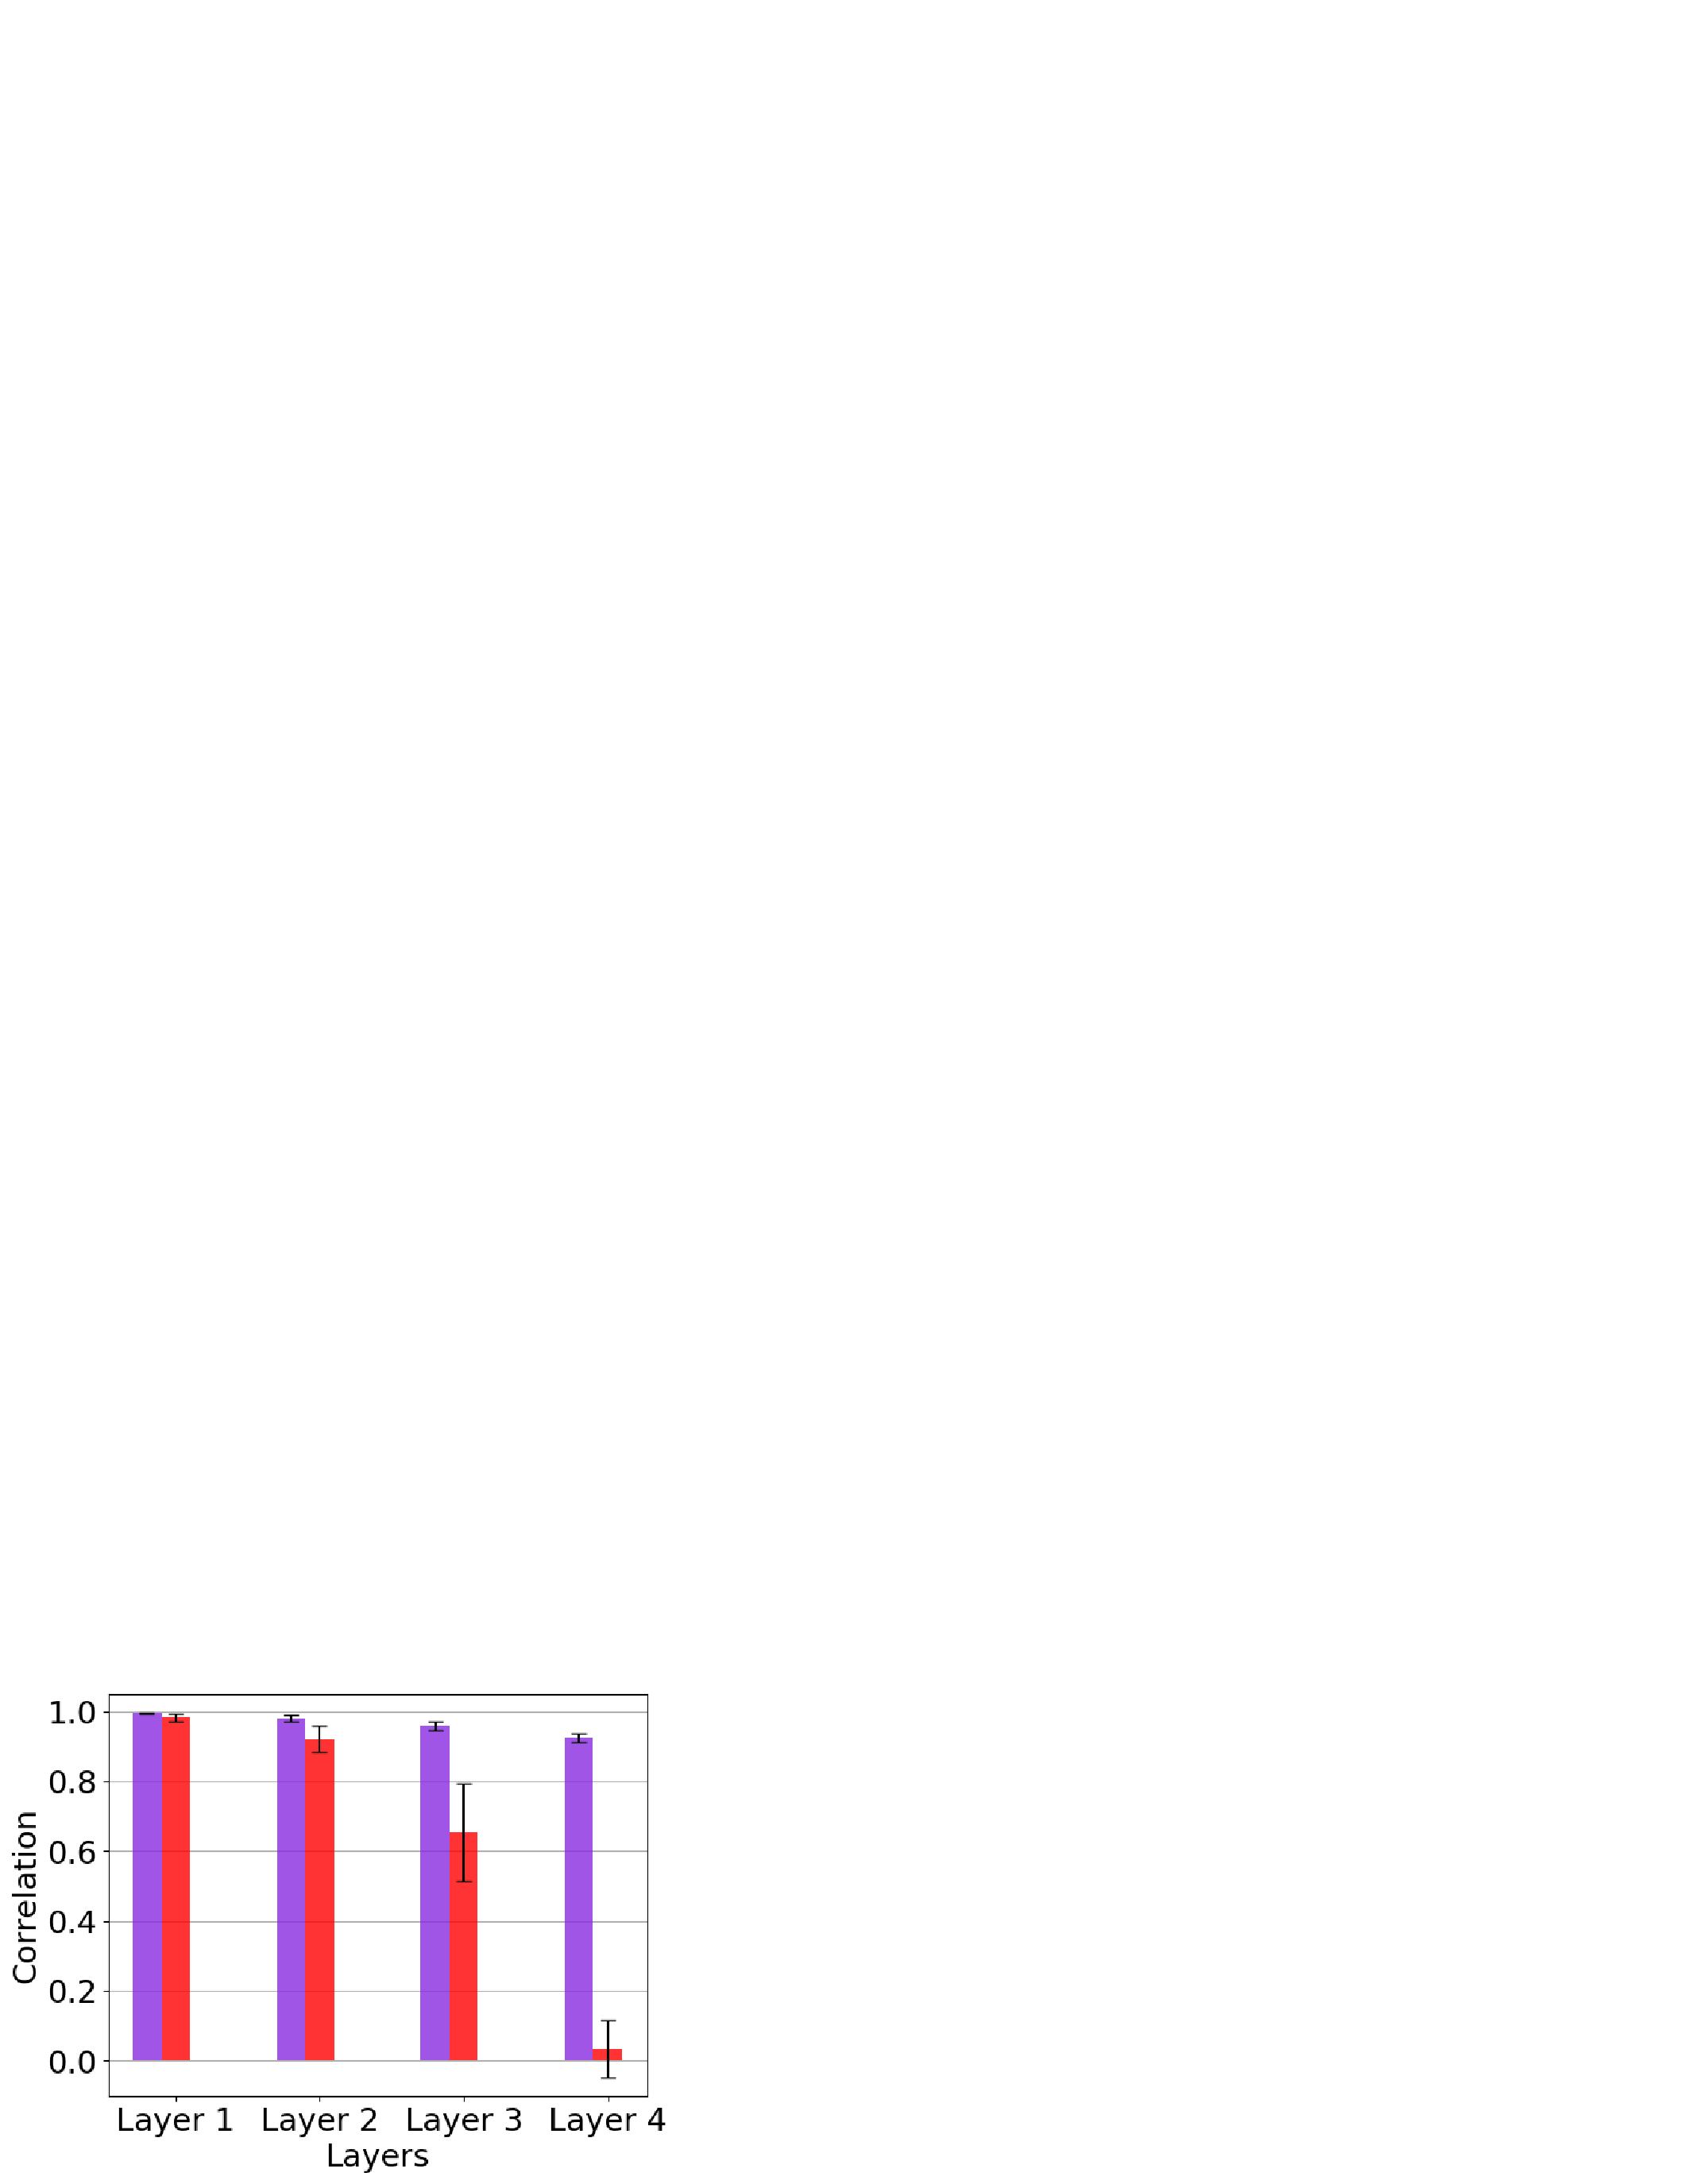}
            \caption{}
            \label{fig:multitask_corr}
        \end{minipage}
    \end{subfigure}
    \vspace{-5pt}
    \caption{Effect of single-task vs multitask training. (\subref{fig:multitask_learning_speed}) Comparison of learning speed of the networks. (\subref{fig:multitask_error}) Comparison of the error in average task performance over all data when multitasking compared to single-tasking (the lack of a bar indicates no error). (\subref{fig:multitask_corr}) Correlation of convolutional layer representations between Tasks $3$ and Tasks $4$ computed using the average representation for each layer across all the data. We again show results for the tasks involving the convolutional network.}
    \label{fig:multitask_diff_init}
    \vspace{-5pt}
\end{figure}
\endgroup

\subsection{Visualization of Meta-Learner}
In Figure~\ref{fig:posterior}, we visualize the predictive distribution of rewards at various trials when varying amount of data has been observed. We see that the predictive distribution is initially uncertain when observing a small amount of rewards for each strategy (which is useful for exploration) and grows certain as more data is observed (which is utilized to be greedy).

\begin{figure}
    \begin{subfigure}[t]{\textwidth}
      \captionsetup{justification=raggedright,singlelinecheck=false,margin=4.33cm}
      \includegraphics[width=0.5\linewidth]{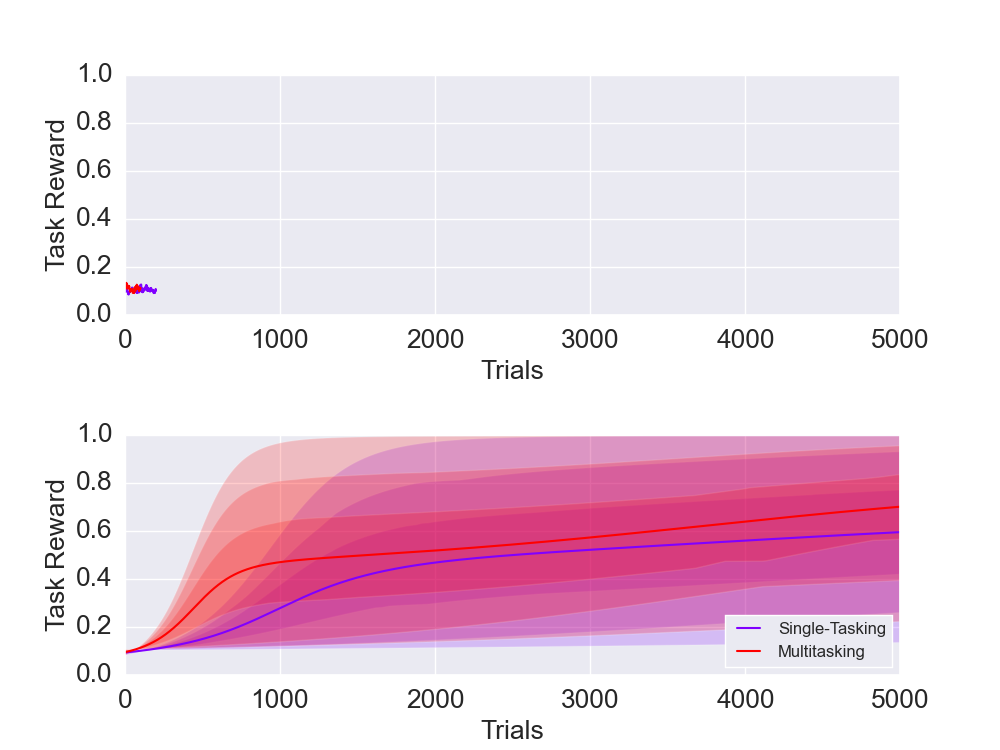}
      \caption{}
      \label{fig:posterior1}
    \end{subfigure}
    \begin{subfigure}[t]{\textwidth}
      \captionsetup{justification=raggedright,singlelinecheck=false,margin=4.33cm}
      \includegraphics[width=0.5\linewidth]{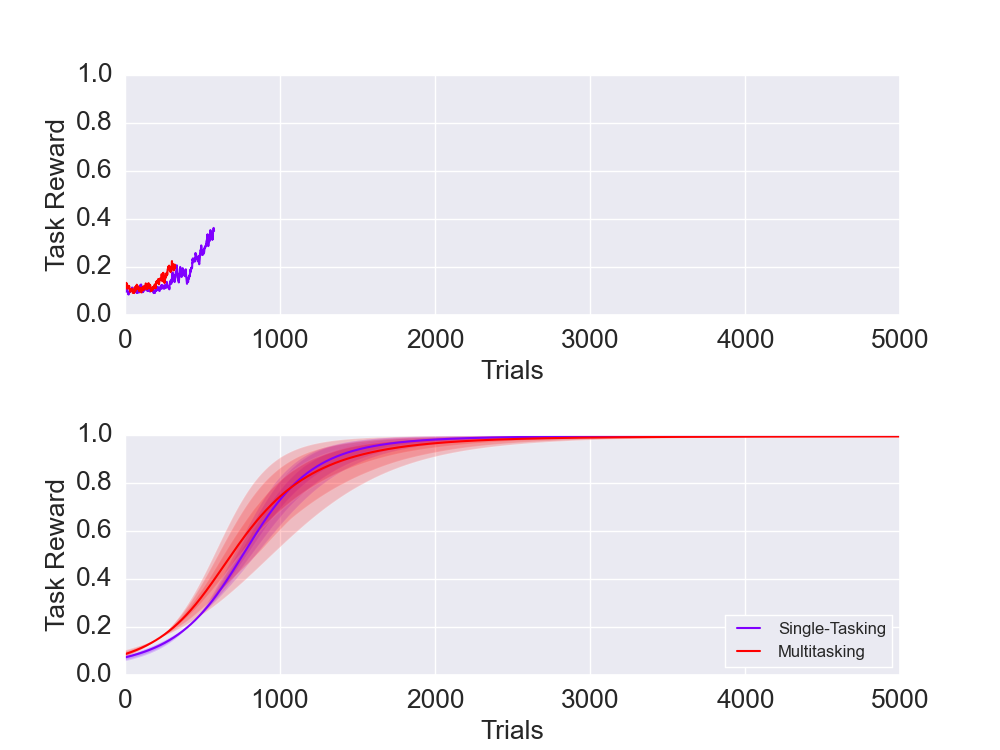}
      \caption{}
      \label{fig:posterior2}
    \end{subfigure}
    \begin{subfigure}[t]{\textwidth}
      \captionsetup{justification=raggedright,singlelinecheck=false,margin=4.33cm}
      \includegraphics[width=0.5\linewidth]{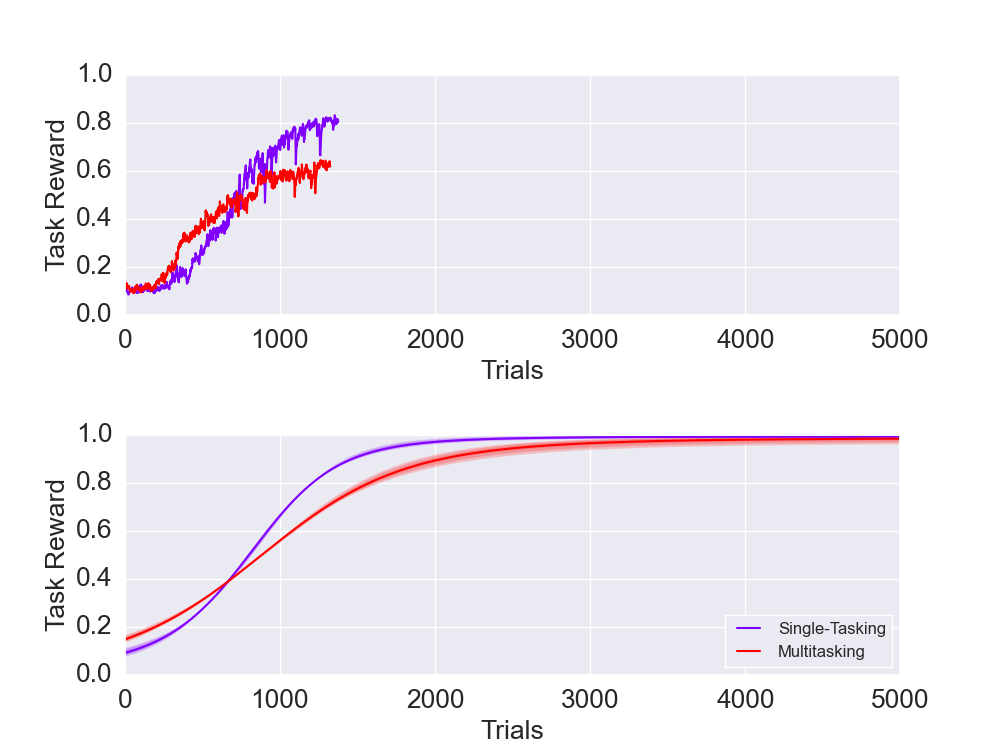}
      \caption{}
      \label{fig:posterior3}
    \end{subfigure}
    \caption{Visualization of actual rewards and predictive distribution of rewards for a specific task. Shaded areas correspond to $\pm 3$ standard deviations around mean. For each of (\subref{fig:posterior1}), (\subref{fig:posterior2}), and (\subref{fig:posterior3}), we show the actual rewards accumulated over trials for each strategy (on top) and the predictive distribution over reward data computed using samples from the posterior distribution over parameters for each strategy given the reward data (on bottom).}
    \label{fig:posterior}
\end{figure}
